# Supplementary material for: A New Korean Text Classification Benchmark for Recognizing the Political Intents in Online Newspapers
Source: arXiv:2311.01712 source file (2023-11-03)
Supplement: Supplementary file 1 [file appendix.tex]

\newpage
\onecolumn
\appendix
\clearpage

\section{Data Labelling Guideline}
\subsection{Labeling Priority}
\begin{enumerate}
    \item \textbf{Intention of the Journalist}
    \begin{itemize}
        \item If the article conveys one side's argument even without the journalist's personal opinion, it is considered as agreeing with that argument.
        \item If both sides of the argument are presented, the quantity of each side's content will be taken into account.
        \item If the article only lists the current situation without taking a side, it should be categorized under the neutral option.
    \end{itemize}
    
    \item \textbf{Policy}
    \begin{itemize}
        \item Upon mentioning policy-related content, it is classified based on the values traditionally pursued by political parties. For example, article that conservative party emphasize welfare policies are classified as liberal.
        \item \textit{Liberal:} Emphasis on public education, other welfare expansions, support for North Korea, expansion of labor rights, etc.
        \item \textit{Conservative:} Emphasis on private education, gifted education (expansion of autonomous private high schools), anti-communism, corporate tax cuts, other corporate support policies, relaxation of inheritance and gift taxes, etc.
    \end{itemize}
    
    \item \textbf{Political Party}
    \begin{itemize}
        \item \textit{Liberal:} Democratic Party, Justice Party
        \item \textit{Conservative:} People Power Party(PPP)
    \end{itemize}
\end{enumerate}

\subsection{Additional Specific Criteria}
\begin{enumerate}
    \item Political Orientation
    \begin{itemize}
        \item \textbf{Label 1}: Strong criticism of the conservative administration or conservative party
        \item \textbf{Label 2}: While not overtly critical, the content opposes the conservative faction
        \item \textbf{Label 3}: Internal conflict (e.g., intra-party disagreements), Equal citation or simple listing of both sides' opinion, Differences between government departments
        \item \textbf{Label 4}: Criticism of the liberal faction
        \item \textbf{Label 5}: Strong criticism of the liberal administration or liberal party
    \end{itemize}
    
    \item The level of Pro-Government
    \begin{itemize}
        \item \textbf{Label 0}: When the government is not mentioned
        \item \textbf{Label 1}: Direct criticism/condemnation of the president (government)
        \item \textbf{Label 2}: Criticism of government policy
        \item \textbf{Label 3}: Internal conflict within the government, Cases where only the current situation is listed without opinion
        \item \textbf{Label 4}: Positive assessment of the government.
        \item \textbf{Label 5}: Strong advocacy for government policies, Promotional publicity of the president
    \end{itemize}
\end{enumerate}

\clearpage
\section{Representative Sentences Classified by the Model}
\subsection{Correctly Categorized Case Examples}

\begin{table}[!htb]
    \centering

    \begin{adjustbox}{width=\textwidth}
    \begin{tabular}{|p{8cm}|p{12cm}|p{0.7cm}|p{0.7cm}|}
        \hline
        \multicolumn{1}{|c|}{\textbf{Article}} & \multicolumn{1}{c|}{\textbf{Translation}} & \multicolumn{1}{c|}{\textbf{Task 1}} & \multicolumn{1}{c|}{\textbf{Task 2}} \\
        \hline
       국힘 "노인 존재 부정하는 민주당 DNA…김은경, 즉각 사퇴해야" 국민의힘은 1일 김은경 더불어민주당 혁신위원장의 '노인 비하' 논란에 대해 노인의 존재를 부정하는 민주당의 DNA 탓이라고 비판했다. 윤재옥 원내대표는 이날 오전 국회에서 열린 원내대책회의에서 "민주당은 2004년 열린우리당 시절부터 입에 담을 수 없는 노인 폄하 발언의 긴 역사를 가진 정당"이라며 "김 위원장이 진정으로 혁신해야 할 것은 이처럼 갈등적 세계관으로 사회 바라보며 표 계산만 앞세워 극단적 국민 분할 지배전략으로 선거에 접근하는 민주당의 구태"이라고 지적했다.그는 회의 후 기자들과 만나 김 위원장에 대해 "민주당의 반응이나 입장을 오늘 지켜볼 것"이라며 "문제를 제기를 했으니 사과하든가 아니면 해명하든가 민주당의 입장이 있을 것이라고 생각한다. 그 입장에 따라 저희 당이 조치할 사안이 있으면 조치하겠다"고 말했다.이철규 사무총장은 회의에서 "김은경 위원장의 현대판 고려장 노인 폄하 발언을 규탄한다"며 "이것은 정쟁이 아니다. 김 위원장의 망언에 대한 타당하고 정당한 지적으로 전쟁으로 무너진 나라를 한강의 기적으로 일으키며 지금 대한민국이 있게 한 세대가 어른신들이다"라고 말했다. 이 사무총장은 "거대 야당의 혁신위원장이라는 분이 혁신을 이끄는 게 아니라 불신을 이끄는 상황이야말로 민주당의 미래를 확실히 보여준다"며 정동영 전 대표, 윤호중 의원, 유시민 전 보건복지부 장관 등 야권 인사들의 과거 노인 비하 발언을 언급했다. 그는 "이렇듯 민주당의 막말이 반복되는 것은 민주당의 DNA가 노인을 폄훼하고 노인의 존재를 부정하는, 또한 대한민국 건국과 번영을 이룩한 세대를 부정하는 망언이라고 생각하지 않을 수 없다"며 "김 위원장은 대국민 사과를 하고 즉각 그 자리에서 내려오라"고 밝혔다.송석준 의원은 "김 위원장이 엄청난 혁신을 제안할 줄 알았는데 이게 무슨 말씀이냐"며 "혁신하라고 했더니 혁신하지 않고 마치 청년이 민주당 편인 줄 착각하는 모습에 기가 막힌다"고 했다.앞서 김 위원장은 지난 30일 '2030 청년좌담회'에서 자신이 아들이 중학생 시절 나눈 대화를 소개하며 "왜 미래가 짧은 분들이 (젊은 사람들과) 1 대 1 표결해야 하느냐"고 발언해 논란이 됐다. & PPP: "Democratic Party's DNA Denies Elderly Existence... Kim Eun-kyung Should Resign Immediately" The People Power Party (PPP) criticized the Democratic Party on the 1st over the controversy of Kim Eun-kyung, Chairman of the Democratic Party's Reform Committee, belittling the elderly. They claimed it's due to the Democratic Party's DNA that denies the existence of the elderly. Yun Jae-ok, the floor leader, stated in a strategic meeting held at the National Assembly that morning, "The Democratic Party has a long history of disparaging the elderly with unspeakable comments since the days of the Our Open Party in 2004." He pointed out that "What Chairman Kim genuinely needs to reform is the Democratic Party's habit of only calculating votes and approaching elections with an extreme strategy of divisive rule." After the meeting, he told reporters regarding Chairman Kim, "We'll see the reaction or position of the Democratic Party today. We believe the Democratic Party will have a stance since we raised the issue. Depending on that stance, our party will take measures if needed." Lee Cheol-gyu, the Secretary-General, during the meeting condemned Kim Eun-kyung's remarks and said, "This isn't about political strife. It's a valid and legitimate criticism of Chairman Kim's absurd remarks. The elderly generation that built the Miracle on the Han River after the war devastation made South Korea what it is today." The Secretary-General highlighted, "It clearly shows the future of the Democratic Party when the chairman of the reform committee of the main opposition party leads distrust instead of reform." He also mentioned previous belittling remarks about the elderly made by figures from the opposition, including former representative Jeong Dong-young, lawmaker Yoon Ho-jung, and former Minister of Health and Welfare Yu Si-min. He added, "Such repeated rude remarks from the Democratic Party can't be thought of as anything other than their DNA belittling and denying the elderly, as well as the generation that achieved the foundation and prosperity of South Korea." He called for Chairman Kim to apologize to the nation and to "step down immediately." Lawmaker Song Seok-jun remarked, "We thought Chairman Kim would propose significant reforms, but what is this? It's baffling to see her mistakenly think the youth side with the Democratic Party instead of innovating." Previously, Chairman Kim, during a '2030 Youth Roundtable' on the 30th, caused controversy by mentioning a conversation she had with her son during his middle school days, asking, "Why do those with a shorter future (referring to the elderly) have to vote 1:1 with young people?"&5 &0 \\
       \hline

    \end{tabular}

    \end{adjustbox}
    \caption{Successful Classification Case1: Based on Political Orientation and Pro-Government Affinity. The model successfully classified Sample 1 based on 'Political Orientation' and 'Pro-Government Affinity' criteria.}
    \label{your_label_here}
\end{table}

\begin{table}[!htb]
    \centering

    \begin{adjustbox}{width=\textwidth}
    \begin{tabular}{|p{8cm}|p{12cm}|p{0.7cm}|p{0.7cm}|}
        \hline
        \multicolumn{1}{|c|}{\textbf{Article}} & \multicolumn{1}{c|}{\textbf{Translation}} & \multicolumn{1}{c|}{\textbf{Task 1}} & \multicolumn{1}{c|}{\textbf{Task 2}} \\
        \hline
       민주당 "윤석열 정부의 정치생명, 원희룡 입에 달려있다" 더불어민주당이 '양평 고속도로 백지화' 관련 원희룡 장관에게 "가짜뉴스 유포 그만하고 사전에 사업 백지화를 재가 받았는지 밝히라"고 촉구했다.강선우 민주당 대변인은 7일 서면브리핑에서 "원희룡 장관이 지금 해야 할 일은 서울-양평 고속도로 종점 변경을 둘러싸고 꼬리를 무는 의문에 답하는 것"이라며 이 같이 밝혔다. 그는 "원희룡 장관이 라디오에 출연해 '민주당이 먼저 발표된 노선대로의 변경을 요청했다'며 우리 당 최재관 지역위원장, 정동균 당시 양평군수에게 책임을 덮어씌웠다"면서 "이는 새빨간 거짓말이다. 주무장관이라는 사람이 국책 사업에 대해서 사실도 확인하지 않고 가짜뉴스를 유포하고 있으니 어처구니없다"고 주장했다. 그는 "팩트를 알려드리겠다. 2년 전에는 변경안 자체가 없었다. 그리고 당시 당정협의를 거쳐 설치하고자 했던 나들목은 강하면 방면이었다"면서 "입을 열 때마다 하나같이 가짜뉴스로 국민을 선동하고 있으니 이쯤되면 국토교통부 장관이 아니라 국민선동부 장관 아닌가. 원희룡 장관, 혹시 롤모델이 괴벨스인가"라고 반문했다. 그는 "사업 백지화에 비판이 쏟아지니 백지화의 책임을 민주당에 덮어씌우려는 원희룡 장관의 나름의 기만술은 처량하고 한심하다"며 "원희룡 장관은 가짜뉴스 유포 그만하고, 사전에 사업 백지화를 윤석열 대통령에게 재가 받았는지나 밝혀라"라고 촉구했다. 그는 "원희룡 장관이 판돈으로 건 것은 자신의 정치생명으로 그치지 않을 것"이라며 "윤석열 정부의 정치생명이 원희룡 장관의 입에 달렸음을 명심하고 성실하게 답하라"고 촉구했다. &The Democratic Party: 'The political life of the Yoon Seok-youl administration hangs on Won Hee-ryong's words. The Democratic Party urged Minister Won Hee-ryong regarding the 'nullification of the Yangpyeong Expressway' to "Stop spreading fake news and clarify whether you have received prior approval for the project nullification." On the 7th, Democratic Party spokesperson Kang Sun-woo stated in a written briefing, "What Minister Won Hee-ryong should be doing now is answering the looming questions surrounding the end-point change of the Seoul-Yangpyeong Expressway." He pointed out, "Minister Won Hee-ryong claimed on the radio that 'the Democratic Party first requested a change to the announced route' and placed blame on our party's regional chairman Choi Jae-gwan and the then-Yangpyeong County head Jung Dong-gyun. This is a blatant lie. It's absurd that a chief minister would spread fake news about a national project without even verifying the facts." He continued, "Let me tell you the facts. There was no proposed change two years ago. And the intersection that was intended to be set up through party-government discussions at that time was towards Gangham. Every time he speaks, he stirs up the public with fake news. At this point, isn't he more of a Minister of Public Instigation than the Minister of Land, Infrastructure, and Transport? Minister Won Hee-ryong, is Goebbels your role model?" He commented, "It's pitiful and pathetic for Minister Won Hee-ryong to try to pin the responsibility of the project nullification on the Democratic Party amidst the mounting criticisms." He urged, "Minister Won Hee-ryong, stop spreading fake news and clarify whether you've received prior approval for the project nullification from President Yoon Seok-yeol." He also emphasized, "The stakes Minister Won Hee-ryong has raised will not just affect his political career." He added, "Keep in mind that the political fate of the Yoon Seok-yeol administration hangs on Minister Won Hee-ryong's words, and provide a sincere answer." &1 &1 \\
       \hline

    \end{tabular}

    \end{adjustbox}
    \caption{Successful Classification Case2: Based on Political Orientation and Pro-Government Affinity.}
    \label{your_label_here}
\end{table}

\clearpage
\subsection{Incorrectly Categorized Case Examples}

The value inside the parentheses represents the classification made by the model. The model tended to misclassify when there were subtle nuances or when contents encompassed two themes simultaneously (e.g., criticism and support or progressive and conservative). In human labeling, if both themes were present, the one that occupied a larger portion was typically chosen for classification. However, as discussed in (Section A.1), our model seems unable to consider such aspects.

\begin{table}[!htb]
    \centering

    \begin{adjustbox}{width=\textwidth}
    \begin{tabular}{|p{8cm}|p{12cm}|p{0.7cm}|p{0.7cm}|}
        \hline
        \multicolumn{1}{|c|}{\textbf{Article}} & \multicolumn{1}{c|}{\textbf{Translation}} & \multicolumn{1}{c|}{\textbf{Task 1}} & \multicolumn{1}{c|}{\textbf{Task 2}} \\
        \hline
        이재명 “야간집회 금지? 집회 때문에 수출 무너졌나” 정부·여당이 야간 집회 금지를 추진하자, 이재명 더불어민주당 대표가 “경제” “안보” 등을 언급하며 반발했다. “집회 때문에 무슨 문제 생긴 것이 있나”라고도 했다.민노총은 지난 16~17일 ‘1박 2일 노숙 시위’를 통해 서울 도심을 치외법권 지역으로 만들고 출퇴근길 교통을 마비시켰다. 일반 시민이라면 과태료나 벌금을 물어야하는 ‘차로 점거’ ‘금연구역 흡연’ ‘쓰레기 무단 투기’ ‘노상 방뇨’ 등을, 민노총 시위대는 아무렇지 않게 저질렀고, 별다른 처벌도 받지 않았다. 이재명 대표는 24일 국회에서 열린 당 최고위에서 정부의 야간 집회 금지 추진에 대해 “집회의 자유마저 박탈하겠다는 의도를 노골적으로 드러내고 있다”며 “헌법정신에 어긋나는 명백한 위헌적 발상이다. 민생경제가 파탄 지경이고, 나라 안보가 백척간두다. 지금 한가하게 집시법 개정을 논할 때인가?”라고 했다. 이재명 대표는 “집회 때문에 수출이 무너졌나? 집회 때문에 민생이 무너졌나? 집회 때문에 민주주의가 파괴되었나? 집회 때문에 무슨 문제 생긴 것이 있나?”라며 “국민의 입을 틀어막는다고 정권의 실정이 가려지지는 않는다. 국정을 위임받았으면 민생과 경제, 안보 문제에 더 집중하시라”고 했다. 이재명 대표는 “집회의 자유를 포함한 표현의 자유는 민주주의를 떠받치는 핵심적인 기본권이다. 이를 제한하려는 어떤 시도도 민주주의에 대한 훼손이고 공격”이라며 “민주당은 윤석열 정권의 민주주의 후퇴 시도를 결코 용납하지 않을 것”이라고 했다. 한편 이날 국민의힘과 정부는 민주노총 건설노조의 1박2일 도심 ‘노숙 집회’를 비판하며 불법집회를 근절하고 심야 집회·시위 금지를 위한 법 개정을 논의하겠다고 밝혔다. 관련 기사 尹 “과거 정부, 불법 집회 법집행 포기… 민노총 행태 방치 안할 것” 야간집회 규제 조항 13년째 입법 공백… ‘24시간 집회’ 방치 한동훈 법무부 장관은 이날 국회에서 열린 ‘공공질서 확립과 국민 권익 보호를 위한 당정협의회’에 참석해 “합법이 아닌 불법 집회는 시민의 일상과 안전을 위협하는 것”이라며 “지난 대통령선거에서 국민들은 불법 집회를 정치적으로 이용하고 방치하는 정부와 불법을 단호히 막고 책임을 묻는 정부 중 후자를 선택했다. 저는 이 상황에 대한 대처로써 국민 선택이 옳았다는 것을 보여드려야 한다고 생각한다”고 했다. & Lee Jae-myung: "A ban on nighttime rallies? Did exports collapse because of the rallies?" When the government and the ruling party pushed for a ban on nighttime demonstrations, Lee Jae-myung, the leader of the Democratic Party, voiced his opposition, mentioning "economy" and "security." He also questioned, "What problems have arisen because of the rallies?" The Korean Confederation of Trade Unions (KCTU) turned the downtown area of Seoul into a lawless zone during their '1-night, 2-day homeless protest' held on the 16th and 17th. This paralyzed the city's traffic. Acts that would normally incur fines or penalties for ordinary citizens, such as 'occupying lanes,' 'smoking in non-smoking areas,' 'illegal dumping of trash,' and 'public urination,' were committed without any repercussions by the KCTU protesters. On the 24th, at a high-level party meeting held in the National Assembly, Representative Lee Jae-myung criticized the government's move to ban nighttime rallies, saying, "It blatantly reveals their intention to deprive even the freedom of assembly. This is a clear unconstitutional thought against the spirit of the Constitution. The livelihood of the people is in tatters, and the country's security is at stake. Is now the time to casually discuss amendments to the Assembly and Demonstration Act?" He added, "Did exports collapse because of the rallies? Did people's lives fall apart because of the rallies? Was democracy destroyed because of the rallies? What problems have arisen because of the rallies?" He further stated, "Hiding the realities of the regime by silencing the people won't work. If you are entrusted with state affairs, focus more on people's livelihood, economy, and security." Representative Lee emphasized, "The freedom of expression, including the freedom of assembly, is a fundamental right that upholds democracy. Any attempt to limit this is a damage and attack on democracy." He continued, "The Democratic Party will never tolerate any attempts by the Yoon Seok-youl administration to backtrack on democracy." Meanwhile, the main opposition Power of the People Party and the government criticized the KCTU's construction labor union for their '1-night, 2-day homeless protest' in downtown Seoul, stating they would discuss amendments to laws to eradicate illegal rallies and ban nighttime protests and demonstrations. Related articles: Yoon stated, "Past governments gave up on enforcing laws against illegal rallies... We won't neglect the KCTU's actions." The clause regulating nighttime demonstrations has been in legislative limbo for 13 years... Neglecting '24-hour demonstrations.' On that day, Minister of Justice Han Dong-hoon, attending the 'Party-Government Consultative Meeting for the Establishment of Public Order and Protection of People's Rights' held at the National Assembly, said, "Illegal rallies that aren't lawful threaten the daily lives and safety of citizens." He added, "In the recent presidential election, people chose a government that decisively stops and holds accountable for illegal actions over a government that politically exploits and neglects illegal rallies. I believe I have to show that the people's choice in this situation was correct."&1(4) &1(1) \\
       \hline

    \end{tabular}

    \end{adjustbox}
    \caption{Unsuccessful Classification Case1: While the model correctly classified the level of Pro-Government(Task 2), it failed in Task1 corresponding to political orientation. The model classified it as 4, indicating 'moderate conservative(4)', but the content of the article is 'liberal(1)'.}
    \label{your_label_here}
\end{table}

\begin{table}[!htb]
    \centering

    \begin{adjustbox}{width=\textwidth}
    \begin{tabular}{|p{8cm}|p{12cm}|p{0.7cm}|p{0.7cm}|}
        \hline
        \multicolumn{1}{|c|}{\textbf{Article}} & \multicolumn{1}{c|}{\textbf{Translation}} & \multicolumn{1}{c|}{\textbf{Task 1}} & \multicolumn{1}{c|}{\textbf{Task 2}} \\
        \hline
       文정부 사드 고의 지연? 與 "안보 주권 포기" 野 "전임 탓 그만" 국민의힘이 문재인 정부 시절의 고고도미사일방어(THAAD·사드) 체계와 관련된 의혹들에 대한 총공세에 나섰다.김기현 대표는 20일 국회에서 열린 당 최고위원회의에서 사드 배치를 위한 환경영향평가를 문재인 정부가 고의 지연시켰다는 의혹과 관련해 “문재인 정권이 철저하게 국민을 기만한 사실이 문서에 의해서 증명되기 시작했다”며 “중국몽과 북한몽에 취해서 안보 농단을 자행한 인사에 대해서는 신분과 지위의 고하를 막론하고 성역없는 감사원의 감사와 수사당국의 수사가 반드시 있어야 할 것”이라고 말했다. 김 대표가 말한 ‘문서’는 국방부가 공개한 ‘환경영향평가 평가협의회 구성 시기 관련 협의 결과에 대한 보고’를 말한다. 보고서에 따르면 2019년 12월 3일 청와대 국가안보실과 국방부ㆍ외교부ㆍ환경부는 경북 성주 사드 기지 환경영향평가를 위한 평가협의회 구성 시점을 논의했는데 2019년 12월 문재인 당시 대통령 방중 등 중국과의 외교 현안을 감안해 위원회 구성을 연기하기로 했다. 해당 문건에는 사드 지연 이유 중 하나로 ‘한·중 간 기존 약속: 3불 합의’가 적혔다. 3불(不)은 ‘사드 추가 배치’, ‘미국의 미사일 방어 체계 참여’, ‘한·미·일 군사 동맹’을 하지 않겠다는 뜻이다. 김 대표는 “문재인 정권은 3불에 대해 철저하게 국가 간 합의나 약속이 아닌 중국의 입장에 불과했다는 주장을 해왔지만 알고 보니 뻔뻔한 거짓말이었다”며 “전대미문의 안보 주권 포기 행위를 결코 묵과할 수 없다”고 말했다. 윤재옥 원내대표는 “문재인 정부 청와대가 사드 발사대 4기의 추가 반입 사실을 군으로부터 구두 보고를 받고도 터무니없는 이유로 보고 누락으로 몰아 국기 문란으로 비화시킨 것이 드러났다”고 주장했다. 2017년 5월 30일 청와대는 “군이 사드 발사대 4기의 추가 반입 보고를 누락했다. 문 대통령이 ‘매우 충격적’이라고 했다”(윤영찬 국민소통수석)며 이른바 ‘사드 보고 누락 사건’ 진상 조사를 대대적으로 했는데, 그 나흘 전에 이미 국방부가 청와대에 구두보고를 했다는 정황이 있다는 주장이다. 윤 원내대표는 또 “문재인 정부는 레이더만이라도 전기를 공급해 달라는 미군의 요구를 묵살했다”며 “문재인 정부가 중국에 잘 보이기 위해 70년 한·미동맹의 역사를 훼손한 것은 분명하다”고도 말했다. 강민국 수석대변인도 논평을 통해 “북한 핵·미사일 위협에 대한 방어 수단이자 대한민국 안보를 위한 사드가 문재인 정부에는 그저 중국의 심기를 거스르는 눈엣가시였을 뿐”이라며 “사드 배치를 둘러싼 문재인 정권의 전방위적 지연·방해 작전이 고스란히 수면위로 떠오르고 있다. 철저히 진상을 밝히겠다”고 말했다. 반면 더불어민주당은 사드 체계가 5년 동안 정상적으로 가동된 만큼 문제 삼을 이유가 없다고 반박했다. 문재인 정부 청와대 국정상황실장을 지낸 윤건영 민주당 의원은 20일 중앙일보와의 통화에서 “주민 반대에도 경찰력 수만명을 배치해서 사드를 가동했던 게 문재인 정부”라며 “당시 환경영향평가법상 주민대표를 선정하지 못했는데 법을 어겨가면서까지 환경영향평가를 할 수는 없었다”고 설명했다. 이어 여권의 사드 환경영향평가 지연 주장에 대해선 “아주 졸렬할 짓이다. 전임 정부 탓 좀 그만했으면 좋겠다”고 말했다.&Moon Administration's intentional delay on THAAD? Ruling party says 'Surrender of security sovereignty', opposition responds 'Stop blaming the predecessor' "The People's Power Party (PPP) launched a full-scale offensive on suspicions related to the Terminal High Altitude Area Defense (THAAD) system during President Moon Jae-in's administration. On the 20th, Representative Kim Ki-hyun, at the party's supreme council meeting in the National Assembly, commented on suspicions that the Moon Jae-in administration intentionally delayed the environmental impact assessment for THAAD deployment. He stated, "Documents are beginning to prove that the Moon Jae-in administration thoroughly deceived the public. Officials, regardless of rank or position, who jeopardized national security for fantasies about China and North Korea should inevitably face an unbiased audit by the Board of Audit and Inspection and an investigation by the authorities." The 'document' that Representative Kim referred to is the 'Report on the consultation results regarding the timing of the Environmental Impact Assessment Review Committee' released by the Ministry of National Defense. According to the report, the Blue House National Security Office, the Ministry of National Defense, the Ministry of Foreign Affairs, and the Ministry of Environment discussed the timing of the Review Committee for the environmental impact assessment of the THAAD base in Seongju, North Gyeongsang Province, on December 3, 2019. They decided to postpone the committee's formation, considering diplomatic issues with China, including President Moon Jae-in's visit to China in December 2019. The document mentioned the '3 Nos Agreement' between South Korea and China as one of the reasons for the THAAD delay. The '3 Nos' refer to not deploying additional THAAD units, not participating in the U.S. missile defense system, and not forming a military alliance between South Korea, the U.S., and Japan. Representative Kim said, "The Moon Jae-in administration has always argued that the '3 Nos' were merely China's position, not a formal agreement between countries. However, it turns out to be a blatant lie. We cannot overlook this unprecedented act of relinquishing national security sovereignty." Yoon Jae-ok, the chief policymaker of the party, claimed, "It was revealed that the Moon Jae-in government's Blue House, after receiving a verbal report from the military about the additional deployment of four THAAD launchers, falsely attributed the omission of the report to absurd reasons, tarnishing national dignity." On May 30, 2017, the Blue House said, "The military omitted the report on the additional deployment of four THAAD launchers. President Moon found it 'very shocking'"(Yoon Young-chan, Senior Secretary for Public Communication). There are allegations that the Ministry of Defense verbally reported to the Blue House four days before the so-called 'THAAD report omission incident' and a thorough investigation was conducted. Chief Policymaker Yoon also added, "The Moon Jae-in administration ignored the U.S. military's request to supply power to the radar. It's clear that the Moon administration damaged the 70-year history of the Korea-U.S. alliance to appease China." Kang Min-kook, the chief spokesperson of the party, also commented, "For the Moon Jae-in administration, THAAD, a defense measure against North Korea's nuclear and missile threats and essential for South Korea's security, was merely an eyesore that upset China. The Moon administration's comprehensive tactics to delay and hinder the deployment of THAAD are becoming evident. We will thoroughly investigate the truth." On the other hand, the Democratic Party refuted, saying there's no reason to make an issue since the THAAD system has been operating normally for five years. Yoon Gun-young, a member of the Democratic Party, who served as the chief of the National Security Situation Room of the Moon Jae-in government's Blue House, explained in a call with JoongAng Ilbo on the 20th, "The Moon Jae-in administration deployed THAAD by stationing tens of thousands of police officers despite opposition from residents. Due to the inability to select resident representatives under the environmental impact assessment law at the time, they couldn't conduct an assessment by breaking the law." He further refuted the ruling party's claim of delaying the THAAD environmental impact assessment, saying, "It's a very sly act. I wish they'd stop blaming the previous administration." &5(3) &0(4) \\
       \hline

    \end{tabular}

    \end{adjustbox}
    \caption{Unsuccessful Classification Case2: Based on Political Orientation and the level of Pro-Government. For Political Orientation (Task 1), even though the Ground Truth is Criticism(5), the model classified it as Moderate(3). Also, based on the level of Pro-Government criterion, despite there being no mention about the current government, resulting in a Ground Truth of None(0), it's being classified as Moderate Advocacy (4).}
    \label{your_label_here}
\end{table}

\clearpage
\section{List of Common Sentences from Articles Classified with High Confidence}
\subsection{Task of Political Orientation}

\begin{table}[!htb]
\centering
 % Adjusting the row spacing
\begin{adjustbox}{width=\textwidth}
\begin{tabular}{m{0.5cm}|m{12cm}|m{11cm}}\hline
\toprule
class              & Comman Sentence of each label in Korean                                                                                                                                         & Translation of comman sentence of each label                                                                                                                                                                                                                                                                                                                                                                                                                                                 \\ 
\hline
\multirow{3}{*}{1} & 정부와 여당을 향해서는 “집권 여당은 국민 생명과 인전을 지키려는 노력을 고사하고 횟집 퍼포먼스를 이어가며 국민 우려를 괴담이라 비난하기 바쁘다”며 “윤석열 대통령은 답해야 한다. 검증조차 안된 결과에 우리 영해와 우리 생명을 통째로 맡길 셈인가”라고 비판했다.                              & Toward the government and the ruling party, he said, "The ruling party is busy putting on a show and denouncing people's concerns as myths, let alone making efforts to protect people's lives and property. Are you willing to entrust our territorial waters and our lives to an unverified outcome?" he criticized.                                                                                                                                                                       \\ 
\cline{2-3}
                   & 더불어민주당이 '양평 고속도로 백지화' 관련 원희룡 장관에게 "가짜뉴스 유포 그만하고 사전에 사업 백지화를 재가 받았는지 밝히라"고 촉구했다.                                                                                                 & The Democratic Party of Korea urged Minister Won Hee-ryong to "stop spreading fake news and reveal whether the project was approved beforehand" in relation to the "Yangpyeong Expressway whiteout.                                                                                                                                                                                                                                                                                          \\ 
\cline{2-3}
                   & 이재명 더불어민주당 대표가 이상민 행정안전부 장관을 향해 “기각 결정문이 면죄부가 될 수 없다”며 “탄핵이 되든 안 되든 정부가 매우 무능하고 무책임하다는 것”이라고 26일 지적했다.                                                                          & Lee Jae-myung, leader of the Democratic Party of Korea, said  "The impeachment decision cannot be an exoneration," toward Minister of the Interior and Safety Lee Sang-min. "Whether it is impeachment or not, it means that the government is very incompetent and irresponsible."                                                                                                                                                                                                          \\ 
\cline{1-3}
\multirow{3}{*}{2} & 2021년 더불어민주당 전당대회 돈봉투 의혹'의 중심에 선 송영길 전 민주당 대표가 22일 프랑스 파리에서 기자회견을 열고 "모든 정치적 책임을 지고 탈당하겠다"고 밝혔다.                                                                                & Former Democratic Party of Korea representative Song Young-gil, who is at the center of the 2021 Democratic Party of Korea National Convention money envelope scandal, held a press conference in Paris, France, on Feb. 22 to announce that he will "take all political responsibility and leave the party."                                                                                                                                                                                \\ 
\cline{2-3}
                   & 민주당은 이날 오후 기자들에게 “오늘 예정된 이재명 대표와 이낙연 전 대표와의 회동 일정은 호우 경보와 그에 따른 수해로 연기한다”고 공지했다.                                                                                                & Today's scheduled meeting with Representative Lee Jae-myung and former Representative Lee Nak-yeon will be postponed due to the heavy rain warning and resulting flooding, the Democratic Party announced to reporters later in the day.                                                                                                                                                                                                                                                     \\ 
\cline{2-3}
                   & 이에 민주당 소속 소병훈 농해수위원장은 "실무상 여러 차례 (여야 의원들이 결의안을) 검토한 것으로 안다"며 "해양수산부는 오염수 해양 투기 이후 문제도 다뤄야 한다. 그 대책을 세우라는 촉구 결의안이라 위원회에서 내야 하지 않을까 싶다"며 결의안을 표결에 부쳤다.                            & In response, Democratic Party member So Byung-hoon, chairman of the Agriculture, Forestry and Fisheries Committee, said, "In practice, I know that lawmakers from the ruling and opposition parties have reviewed the resolution several times," adding, "The Ministry of Oceans and Fisheries should also deal with the problem after dumping polluted water into the sea. It is a resolution calling for measures to be taken, so I think it should be tabled by the committee," he said.  \\ 
\cline{1-3}
\multirow{3}{*}{3} & 북한이 '전승절'(한국전쟁 정전협정체결일·27일) 70주년을 맞아 방북 중인 중국 당 및 정부대표단을 직접 접견하고 연회에 초대했다.                                                                                                      & On the 70th anniversary of "Jeonseungjeol" (the 27th anniversary of the signing of the Korean War armistice), North Korea hosted a visiting Chinese party and government delegation and invited them to a banquet.                                                                                                                                                                                                                                                                           \\ 
\cline{2-3}
                   & 반면 한국 정부는 전날 일본을 화이트리스트에 복귀시키는 내용의 '전략물자 수출입 고시'를 관보에 게재한 바 있다.                                                                                                                 & On the other hand, the South Korean government had published a "Notice on Import and Export of Strategic Goods" in the Official Gazette the day before, reinstating Japan to the whitelist.                                                                                                                                                                                                                                                                                                  \\ 
\cline{2-3}
                   & 여야는 13일, 윤석열 대통령이 전날 기시다 후미오 일본 총리와 한 한-일 정상회담에서 “국제원자력기구(IAEA)의 발표 내용을 존중한다”며 일본 정부의 후쿠시마 원자력발전소 오염수 방류를 기정사실화한 것을 두고 공방을 벌였다.                                                 & The ruling and opposition parties sparred over President Yoon Seok-yeol's decision to end the Japanese government's discharge of contaminated water from the Fukushima Daiichi nuclear power plant, saying he "respects the announcement of the International Atomic Energy Agency (IAEA)" during a bilateral meeting with Japanese Prime Minister Fumio Kishida the day before.                                                                                                             \\ 
\cline{1-3}
\multirow{3}{*}{4} & 김기현 국민의힘 대표는 지난 5일 울산에서 기자들과 만나 "IAEA가 일본의 후쿠시마 오염수 방류 계획이 국제 안전기준에 부합한다는 보고서를 제출했다"며 "(야당의) 오염수 괴담 선동은 윤석열 정부 타도를 위한 징검다리이자 수단으로 이용하려는 것"이라고 야당을 비판했다.                         & The IAEA has submitted a report stating that Japan's plan to discharge contaminated water from Fukushima meets international safety standards, Kim Ki-hyun of the People's Power told reporters in Ulsan on May 5. "The opposition's incitement of the contaminated water scandal is an attempt to use it as a stepping stone to overthrow the Yoon Seok-yeol government."                                                                                                                   \\ 
\cline{2-3}
                   & 이어 “이재명 대표가 국면전환용 장외집회 연설까지 하면서 이토록 ‘김남국 일병 구하기’에 매달리는 이유가 도대체 뭔가? 이재명 대표는 도대체 김남국 의원에게 무슨 약점이 잡힌 거냐? 김남국의 코인자산이 김남국의 개인 것이 아니라 대선자금용 돈세탁이었다는 세간의 의혹이 사실인 건가”라고 지적했다.           & Why is Representative Lee Jae-myung so obsessed with 'saving Private Kim Nam-kook' while even giving a speech at an over-the-counter rally to change the situation? What kind of weakness did Representative Lee Jae-myung have against Kim Nam-kook? Is it true that the public's suspicion that Kim Nam-kook's coin assets did not belong to Kim Nam-kook but were laundered for presidential election funds? he said.                                                                     \\ 
\cline{2-3}
                   & 윤 원내대표는 "어민과 시장 상인은 급락한 수산물 소비로 텅 빈 시장을 지키며 살려달라 아우성이다. 이 틈을 탄 담합으로 천일염 가격이 불합리하게 올랐고 선동이 만든 사재기로 국민만 피해를 보고 있다"며 "민주당의 극단적 괴담 선동으로 이득을 보는 건 사법리스크로 궁지에 몰린 민주당과 이재명 대표"라고 주장했다. & Representative Yun said "Fishermen and market vendors are crying out to save their markets, which are empty due to plummeting seafood consumption. The price of sea salt has risen unreasonably due to collusion, and only the public is suffering from the hoarding created by the demagoguery."  and "It is the Democratic Party and Representative Lee Jae-myung who are benefiting from the demagoguery of the Democratic Party's extreme myths."                                        \\ 
\hline
\multirow{3}{*}{5} & 윤석열 대통령은 13일 문재인 정부에서 연간 2조원 가까이 늘어난 민간 단체 보조금에 대해 “지난 정부 때 제대로 된 관리, 감독 시스템이 없어 도덕적 해이와 혈세 누수가 만연했다”며 보조금 관리 투명성을 강화하겠다고 밝혔다.                                                  & President Yun Seok-yeol said on Wednesday that the Moon Jae-in administration will strengthen transparency in subsidy management, saying, "Moral hazard and tax leakage were rampant during the last government due to the lack of a proper management and supervision system," referring to the nearly 2 trillion won in annual subsidies to private organizations.                                                                                                                         \\ 
\cline{2-3}
                   & 국민의힘은 21일 "더불어민주당의 단골메뉴 '가짜뉴스'는 결국 '악의 씨앗'이 돼 온 나라를 멍들게 하고 있다"며 "가짜뉴스와의 전쟁을 선포한다"고 천명했다.                                                                                        & The Democratic Party's regular menu, 'fake news,' has become a 'seed of evil' and is bruising the entire country, the People's Power said on Nov. 21, declaring a war against fake news.                                                                                                                                                                                                                                                                                                     \\ 
\cline{2-3}
                   & 그는 “북한은 어제도 탄도미사일을 발사했는데 한미일은 이를 강력히 규탄한다”고 말했다.                                                                                                                                & North Korea launched a ballistic missile yesterday, which the United States, South Korea and Japan strongly condemn, he said.                                                                                                                                                                                                                                                                                                                                                                \\
\bottomrule
\end{tabular}
\end{adjustbox}
\end{table}

%%%%%%%%%%%%%%%%%%%%%%%%%%%%%%%%%%
\clearpage
\subsection{Task of Pro-government}

\begin{table}[!htb]
\centering
 % Adjusting the row spacing
\begin{adjustbox}{width=\textwidth}
\begin{tabular}{m{0.5cm}|m{11cm}|m{11cm}}\hline
\toprule
class            & Comman Sentence of each label in Korean                                                                                                                                               & Translation of comman sentence of each label                                                                                                                                                                                                                                                                                                                                                                                                                                                         \\ 
\hline
\multirow{4}{*}{1} & 이 대표는 이날 국회에서 열린 최고위원회의에서 “탄핵이 기각됐다고 해서 아무 책임이 없다는 뜻이 아니다”라며 “문제는 정부와 여당의 태도”라고 비판했다.                                                                                                 & The fact that the impeachment was dismissed does not mean that there is no responsibility, Lee told the National Assembly's top committee, criticizing the government and the ruling party's attitude.                                                                                                                                                                                                                                                                                               \\ 
\cline{2-3}
                   & 이 원내대변인은 “심지어 국민의 불안과 우려에 대해서는 한마디 언급조차 없었다. 말로는 국민의 건강과 안전을 최우선으로 한다고 했지만, 윤석열 대통령은 오늘로써 대통령에게 부여된 국민안전에 대한 책임을 완전히 포기한 것”이라고 거듭 강조했다.                                               & There was not even a single mention of the people's anxiety and concern, Lee said. He said he would prioritize the health and safety of the people, but today, he has completely abdicated his responsibility for the safety of the people," Yoon reiterated.                                                                                                                                                                                                                                        \\ 
\cline{2-3}
                   & 제3지대 신당 창당을 추진 중인 금태섭 전 의원이 윤석열 대통령의 '이권 카르텔' 발언에 대해 "책임을 모면하기 위한 '알리바이 정치'"라고 비판했다.                                                                                                  & Former lawmaker Geum Tae-seop, who is pushing for the creation of a third party, criticized President Yoon Seok-yeol's "cartel of interests" remarks, calling them "alibi politics to avoid responsibility.                                                                                                                                                                                                                                                                                          \\ 
\cline{2-3}
                   & 이어 “방류 점검 과정에서 한국 전문가가 참여하면 우리 국민의 우려가 깨끗이 씻깁니까. 방사성 물질 농도가 기준치를 초과할 때 즉시 방류를 중단해야 한다는 말은 너무나 당연한 것 아닙니까”라고 반문하며 “윤석열 대통령은 몇 가지 조건을 붙였지만 일본의 오염수 방류를 막을 생각이 조금도 없음을 분명히 보여주었다”고 비판했다. & Doesn't the involvement of South Korean experts in the discharge inspection process wash away the concerns of the Korean people, and isn't it a given that the discharge must be stopped immediately when the concentration of radioactive material exceeds the threshold? he asked, criticizing, "President Yoon has clearly shown that he has no intention of stopping Japan's discharge of contaminated water, even though he has attached some conditions."                                      \\ 
\hline
\multirow{4}{*}{2} & 시찰단이 현장에서 오염수 처리에 대해 설명을 듣고 난 이후에 즉각적인 문제제기를 하지 않는다면, 한국 정부가 추후에 이를 반대할 명분이 약해지기 때문이다.                                                                                                & If the inspectors don't raise the issue immediately after hearing about the treatment of contaminated water at the site, the South Korean government will have a weaker argument against it later.                                                                                                                                                                                                                                                                                                   \\ 
\cline{2-3}
                   & 여기에 한국 정부가 시찰단 활동도 시작하기 전에 '오염수'라는 용어를 '처리수'로 바꾸기 위해 검토 작업에 착수했다는 보도까지 나오면서, 한국 시찰단 파견은 안전성 검증이 아닌, 오염수 방류에 대한 한국 내 여론을 잠재우고 일본의 방류를 허용하기 위한 이른바 '절차적 요식행위' 아니냐는 지적도 나오고 있다.          & In addition, there are reports that the South Korean government has begun reviewing the term "contaminated water" to replace it with "treated water" before the mission has even begun, raising concerns that the mission is not a safety check, but rather a "procedural gimmick" to silence public opinion in South Korea about the discharge of contaminated water and allow Japan to discharge it.                                                                                               \\ 
\cline{2-3}
                   & 정부·여당이 사안마다 감사원과 검찰을 동원하면서 여당 내에서조차 우려의 목소리가 나온다.                                                                                                                                     & There are concerns even within the ruling party as the government mobilizes auditors and prosecutors for each case.                                                                                                                                                                                                                                                                                                                                                                                  \\ 
\cline{2-3}
                   & 참사가 발생하고 1년 가까운 시간이 지나서야 감사원이 감사에 나서는 셈이어서 ‘늑장 감사’라는 비판을 피할 수 없게 됐다.                                                                                                                  & The fact that the auditors waited nearly a year after the tragedy to conduct their audit has led to criticisms of a "wolf in sheep's clothing" audit.                                                                                                                                                                                                                                                                                                                                                \\ 
\hline
\multirow{4}{*}{3} & 한국갤럽이 30일 발표한 조사에서 윤석열 대통령 지지율이 36\%로 나타났다. 윤 대통령의 직무수행을 긍정 평가한 이유, 부정 평가한 이유 1위는 모두 ‘외교’였다.                                                                                          & President Yoon Seok-yul's approval rating is 36 percent, according to a survey released by Gallup Korea on Tuesday. "Diplomacy" was the top reason for both positive and negative ratings of President Yoon's job performance.                                                                                                                                                                                                                                                                       \\ 
\cline{2-3}
                   & 합동참모본부는 5일 “지난 5월 31일부터 시작한 북한 우주발사체 등 잔해물 탐색 및 인양작전을 7월 5일부로 종료했다”며 “감시 전력을 운용해 북한의 발사체가 발사된 순간부터 추적한 후 잔해물 낙하구역을 설정했고, 해군 함정, 항공기, 심해 잠수사 등을 투입해 36일 간의 탐색 및 인양 작전을 수행했다”고 설명했다.    & The search and retrieval operation for debris from the North Korean space launch vehicle that began on May 31 ended on July 5, the Joint Chiefs of Staff said on Friday, explaining that "we used surveillance power to track the North Korean launch vehicle from the moment it was launched, set up a debris drop zone, and conducted a 36-day search and retrieval operation using naval ships, aircraft, and deep-sea divers."                                                                   \\ 
\cline{2-3}
                   & 김 차장은 “첨단 산업과 방위산업, 인프라와 인적교류 등 다양한 분야의 실질적인 협력 증진 방안, 우크라이나 정세와 북핵·미사일 위협 등 국제적·지역적 위협이 되는 안보 정세에 대해 논의했다”고 부연했다                                                                     & We discussed ways to promote practical cooperation in various fields such as high-tech and defense industries, infrastructure and people-to-people exchanges, and the security situation that poses international and regional threats, including the situation in Ukraine and the North Korean nuclear and missile threats, Kim added.                                                                                                                                                              \\ 
\cline{2-3}
                   & 윤석열 대통령과 부인 김건희 여사는 정전협정 70주년을 맞은 27일 부산 유엔기념공원을 찾아 데임 신디 키로 뉴질랜드 총독 부부, 자비에 베텔 룩셈부르크 총리 등 유엔 참전국 정부대표단과 함께 역대 대통령 최초로 유엔군 위령탑에 참배했다.                                                 & President Yun Suk-yeol and his wife, Kim Gun-hee, visited the UN Memorial Park in Busan on the 70th anniversary of the Armistice Agreement, and became the first president to visit the UN Soldiers Memorial Tower, along with a delegation of governments from UN participating countries, including New Zealand Governor-General Damien Cindy Kiro and Luxembourg Prime Minister Xavier Bettel.                                                                                                    \\ 
\hline
\multirow{3}{*}{4} & 박 차장은 "일본 측 방류 실시계획의 현실성을 평가할 때 핵심은 2·3차 시료를 채취한 일반 저장탱크 속 오염수 농도가 아니라, 1차 시료를 채취한 K4 탱크에서 정확하게 핵종 농도를 파악해내는 능력이라고 보아야 한다"고 강조했다                                                      & The key to assessing the realism of Japan's discharge plan is the ability to accurately determine the nuclide concentrations in the K4 tank, where the first sample was taken, rather than the contaminated water concentrations in the general storage tanks where the second and third samples were taken, Park said.                                                                                                                                                                              \\ 
\cline{2-3}
                   & 정부 또한 사업 정상화를 위한 전문가 검증과 주민 의견 수렴 과정에 민주당이 전문가를 추천한다면 함께 논의하겠다는 입장"이라고 밝혔다.                                                                                                           & The government is also willing to discuss with the Democratic Party if it recommends experts in the process of verifying experts and collecting public opinions to normalize business."                                                                                                                                                                                                                                                                                                              \\ 
\cline{2-3}
                   & 박 의원은 "윤석열 정부는 그러한 경험을 바탕으로 방송의 공정성, 미디어의 공정성 확보를 위한 차원에서 이동관을 내정했다"며 이 내정자 인사는 방송탄압 아닌 방송의 공정성을 되찾으려는 조치라고 주장했다.                                                                     & Based on that experience, the Yoon administration has nominated a minister to ensure fairness in broadcasting and fairness in the media, Park said, arguing that the appointment is a measure to restore fairness in broadcasting, not to suppress it.                                                                                                                                                                                                                                               \\ 
\hline
\multirow{4}{*}{5} & 비공개 회의에서도 윤 대통령은 "말도 안 되는 정치 보조금은 없애고, 경제 보조금은 살리고, 사회 보조금은 효율화‧합리화 해야 한다"고 했다고 이도운 대변인은 전했다                                                                                          & In a closed-door meeting, president Yun said, "We need to eliminate ridiculous political subsidies, save economic subsidies, and streamline and rationalize social subsidies," according to spokesman Lee Do-woon.                                                                                                                                                                                                                                                                                   \\ 
\cline{2-3}
                   & 윤석열 대통령은 1일 최근 아파트 현장에서 드러난 부실 시공을 질타하며 "국민 안전을 도외시한 이권 카르텔은 반드시 깨부숴야 한다"고 강조했다.                                                                                                      & President Yoon Seok-yeol on Jan. 1 criticized faulty construction at recent apartment sites and emphasized that "interest cartels that ignore public safety must be broken."                                                                                                                                                                                                                                                                                                                         \\ 
\cline{2-3}
                   & 윤 대통령은 “어제 북한의 대륙간탄도미사일(ICBM) 발사를 강력히 규탄하고 북한이 한반도와 국제사회의 평화와 안전을 위협하는 핵, 미사일 개발을 즉시 중단하도록 단호히 대응해 나가기로 했다”며 “북한 불법 노동자 파견과 사이버 활동을 차단하면서 북한 인권 상황 개선을 위한 공동 노력을 배가해 나가기로 했다”고 말했다.   & We strongly condemned yesterday's launch of an intercontinental ballistic missile (ICBM) by North Korea and decided to respond decisively to ensure that Pyongyang immediately stops its nuclear and missile programs that threaten the peace and security of the Korean Peninsula and the international community, president Yun said. "We will redouble our joint efforts to improve the human rights situation in North Korea by blocking the dispatch of illegal workers and cyber activities."  \\ 
\cline{2-3}
                   & 윤 대통령은 북한 핵미사일 위협과 함께 우크라이나 전쟁을 언급하며 "이러한 위협들을 만들어 내고 조장하는 것은 바로 전체주의와 권위주의 세력"이라고 했다.                                                                                                & It is the totalitarian and authoritarian forces that create and promote these threats, president Yun said, referring to the war in Ukraine along with the North Korean nuclear and missile threats.                                                                                                                                                                                                                                                                                                  \\
\bottomrule
\end{tabular}
\end{adjustbox}
\end{table}

\clearpage
\section{List of Common Vocabulary from Articles Classified with High Confidence}

\vspace{30pt}
\begin{table}[h]
\centering
 % Adjusting the row spacing
\begin{adjustbox}{width=\textwidth}
\begin{tabular}{|c|c|c|c|c|c|} 
\hline
   & \multicolumn{5}{c|}{Political Orientation}                                                                                                                                    \\ 
\cline{2-6}
Rank   & Class 1                                                                                                         & Class 2                                                                                                          & Class 3                                                                                                     & Class 4                                                                                                      & Class 5                                                                                                      \\ 
\hline
1  & \begin{tabular}[c]{@{}c@{}}이 (110)\\Last name of some\\politicians or This\\(Yi)\end{tabular}                   & \begin{tabular}[c]{@{}c@{}}이 (284)\\Last name of some\\politicians or This\\(Yi)\end{tabular}                    & \begin{tabular}[c]{@{}c@{}}전 (301)\\Ex \\(jeon)\end{tabular}                                                & \begin{tabular}[c]{@{}c@{}}했다. (336)\\did \\(haessda)\end{tabular}                                           & \begin{tabular}[c]{@{}c@{}}했다. (95)\\did \\(haessda)\end{tabular}                                            \\ 
\hline
2  & \begin{tabular}[c]{@{}c@{}}윤석열 (80)\\Name of Korea\\president\\(yunseogyeol)\end{tabular}                       & \begin{tabular}[c]{@{}c@{}}전 (281)\\Ex \\(jeon)\end{tabular}                                                     & \begin{tabular}[c]{@{}c@{}}있다. (249)\\be \\(issda)\end{tabular}                                             & \begin{tabular}[c]{@{}c@{}}전 (268)\\Ex \\(jeon)\end{tabular}                                                 & \begin{tabular}[c]{@{}c@{}}윤 (72)\\Last name of some\\politicians \\(yun)\end{tabular}                       \\ 
\hline
3  & \begin{tabular}[c]{@{}c@{}}있다. (69)\\be \\(issda)\end{tabular}                                                  & \begin{tabular}[c]{@{}c@{}}있다. (256)\\be \\(issda)\end{tabular}                                                  & \begin{tabular}[c]{@{}c@{}}했다. (202)\\did \\(haessda)\end{tabular}                                          & \begin{tabular}[c]{@{}c@{}}윤 (250)\\Last name of some\\politicians \\(yun)\end{tabular}                      & \begin{tabular}[c]{@{}c@{}}대통령은 (62)\\President is \\(daetongryeongeun)\end{tabular}                         \\ 
\hline
4  & \begin{tabular}[c]{@{}c@{}}했다. (68)\\did \\(haessda)\end{tabular}                                               & \begin{tabular}[c]{@{}c@{}}했다. (214)\\did \\(haessda)\end{tabular}                                               & \begin{tabular}[c]{@{}c@{}}이 (182)\\Last name of some\\politicians or This\\(Yi)\end{tabular}               & \begin{tabular}[c]{@{}c@{}}이 (236)\\Last name of some\\politicians or This\\(Yi)\end{tabular}                & \begin{tabular}[c]{@{}c@{}}이 (40)\\Last name of some\\politicians or This\\(Yi)\end{tabular}                 \\ 
\hline
5  & \begin{tabular}[c]{@{}c@{}}윤 (61)\\Last name of some\\politicians \\(yun)\end{tabular}                          & \begin{tabular}[c]{@{}c@{}}민주당 (123)\\The name of Korea liberal party \\(minjudang)\end{tabular}                 & \begin{tabular}[c]{@{}c@{}}윤 (161)\\Last name of some\\politicians \\(yun)\end{tabular}                     & \begin{tabular}[c]{@{}c@{}}있다. (196)\\be \\(issda)\end{tabular}                                              & \begin{tabular}[c]{@{}c@{}}대표는 (39)\\Representative is \\(daepyoneun)\end{tabular}                           \\ 
\hline
6  & \begin{tabular}[c]{@{}c@{}}전 (58)\\Ex \\(jeon)\end{tabular}                                                     & \begin{tabular}[c]{@{}c@{}}대표는 (115)\\Representative is \\(daepyoneun)\end{tabular}                              & \begin{tabular}[c]{@{}c@{}}말했다. (128)\\Said \\(malhaessda)\end{tabular}                                     & \begin{tabular}[c]{@{}c@{}}말했다. (171)\\Said \\(malhaessda)\end{tabular}                                      & \begin{tabular}[c]{@{}c@{}}김 (39)\\Last name of some\\politicians\\(kim)\end{tabular}                        \\ 
\hline
7  & \begin{tabular}[c]{@{}c@{}}비판했다. (54)\\Criticized \\(bipanhaessda)\end{tabular}                                 & \begin{tabular}[c]{@{}c@{}}더불어민주당 (105)\\The full name of Korea liberal party \\(deobureominjudang)\end{tabular} & \begin{tabular}[c]{@{}c@{}}대통령은 (124)\\President is \\(daetongryeongeun)\end{tabular}                       & \begin{tabular}[c]{@{}c@{}}김 (165)\\Last name of some\\politicians\\(kim)\end{tabular}                       & \begin{tabular}[c]{@{}c@{}}말했다. (37)\\Said \\(malhaessda)\end{tabular}                                       \\ 
\hline
8  & \begin{tabular}[c]{@{}c@{}}말했다. (52)\\Said \\(malhaessda)\end{tabular}                                          & \begin{tabular}[c]{@{}c@{}}윤 (104)\\Last name of some\\politicians \\(yun)\end{tabular}                          & \begin{tabular}[c]{@{}c@{}}윤석열 (116)\\Name of Korea\\president\\(yunseogyeol)\end{tabular}                  & \begin{tabular}[c]{@{}c@{}}국민의힘 (156)\\The full name of Korea conservative party\\(gukminuihim)\end{tabular} & \begin{tabular}[c]{@{}c@{}}전 (28)\\Ex \\(jeon)\end{tabular}                                                  \\ 
\hline
9  & \begin{tabular}[c]{@{}c@{}}대통령이 (50)\\President is \\(daetongryeongi)\end{tabular}                              & \begin{tabular}[c]{@{}c@{}}이재명 (103)\\Name of a\\politician\\(ijaemyeong)\end{tabular}                           & \begin{tabular}[c]{@{}c@{}}의원은 (106)\\Member of a legislative assembly is\\(uiwoneun)\end{tabular}          & \begin{tabular}[c]{@{}c@{}}대통령은 (153)\\President is \\(daetongryeongeun)\end{tabular}                        & \begin{tabular}[c]{@{}c@{}}국민의힘 (26)\\The full name of Korea conservative party\\(gukminuihim)\end{tabular}  \\ 
\hline
10 & \begin{tabular}[c]{@{}c@{}}의원은 (46)\\Member of a legislative assembly is\\(uiwoneun)\end{tabular}               & \begin{tabular}[c]{@{}c@{}}의원은 (102)\\Member of a legislative assembly is\\(uiwoneun)\end{tabular}               & \begin{tabular}[c]{@{}c@{}}김 (102)\\Last name of some\\politicians\\(kim)\end{tabular}                      & \begin{tabular}[c]{@{}c@{}}윤석열 (126)\\Name of Korea\\president\\(yunseogyeol)\end{tabular}                   & \begin{tabular}[c]{@{}c@{}}싱 (25)\\Last name of the Chinese ambassador\\(xing)\end{tabular}                  \\ 
\hline
11 & \begin{tabular}[c]{@{}c@{}}대표는 (45)\\Representative is \\(daepyoneun)\end{tabular}                              & \begin{tabular}[c]{@{}c@{}}윤석열 (96)\\Name of Korea\\president\\(yunseogyeol)\end{tabular}                        & \begin{tabular}[c]{@{}c@{}}열린 (99)\\Open\\(yeollin)\end{tabular}                                            & \begin{tabular}[c]{@{}c@{}}대표는 (123)\\Representative is \\(daepyoneun)\end{tabular}                          & \begin{tabular}[c]{@{}c@{}}밝혔다. (24)\\Revealed\\(balkhyeossda)\end{tabular}                                  \\ 
\hline
12 & \begin{tabular}[c]{@{}c@{}}김 (43)\\Last name of some\\politicians\\(kim)\end{tabular}                           & \begin{tabular}[c]{@{}c@{}}말했다. (91)\\Said \\(malhaessda)\end{tabular}                                           & \begin{tabular}[c]{@{}c@{}}대통령이 (95)\\President is \\(daetongryeongi)\end{tabular}                          & \begin{tabular}[c]{@{}c@{}}의원은 (119)\\Member of a legislative assembly is\\(uiwoneun)\end{tabular}           & \begin{tabular}[c]{@{}c@{}}있다. (22)\\be \\(issda)\end{tabular}                                               \\ 
\hline
13 & \begin{tabular}[c]{@{}c@{}}정부의 (40)\\Of government\\(jeongbuui)\end{tabular}                                    & \begin{tabular}[c]{@{}c@{}}김 (88)\\Last name of some\\politicians\\(kim)\end{tabular}                            & \begin{tabular}[c]{@{}c@{}}함께 (86)\\Together\\(hamkke)\end{tabular}                                         & \begin{tabular}[c]{@{}c@{}}오염수 (114)\\Contaminated water\\(oyeomsu)\end{tabular}                             & \begin{tabular}[c]{@{}c@{}}보조금 (21\\Subsidy\\(bojogeum)\end{tabular}                                         \\ 
\hline
14 & \begin{tabular}[c]{@{}c@{}}대통령 (39)\\President\\(daetongryeong)\end{tabular}                                    & \begin{tabular}[c]{@{}c@{}}대표가 (81)\\Representative is \\(daepyoga)\end{tabular}                                 & \begin{tabular}[c]{@{}c@{}}북한 (81)\\North Korea\\(bukhan)\end{tabular}                                      & \begin{tabular}[c]{@{}c@{}}대통령이 (99)\\President is \\(daetongryeongi)\end{tabular}                           & \begin{tabular}[c]{@{}c@{}}윤석열 (20)\\Name of Korea\\president\\(yunseogyeol)\end{tabular}                    \\ 
\hline
15 & \begin{tabular}[c]{@{}c@{}}밝혔다. (38)\\Revealed\\(balkhyeossda)\end{tabular}                                     & \begin{tabular}[c]{@{}c@{}}대통령이 (72)\\President is \\(daetongryeongi)\end{tabular}                               & \begin{tabular}[c]{@{}c@{}}밝혔다. (75)\\Revealed\\(balkhyeossda)\end{tabular}                                 & \begin{tabular}[c]{@{}c@{}}민주당 (93)\\The name of Korea liberal party \\(minjudang)\end{tabular}              & \begin{tabular}[c]{@{}c@{}}정부 (18)\\Government\\(jeongbu)\end{tabular}                                       \\ 
\hline
16 & \begin{tabular}[c]{@{}c@{}}대통령은 (38)\\President is \\(daetongryeongeun)\end{tabular}                            & \begin{tabular}[c]{@{}c@{}}국회 (66)\\National assembly\\(gukhoe)\end{tabular}                                     & \begin{tabular}[c]{@{}c@{}}민주당 (75)\\The name of Korea liberal party \\(minjudang)\end{tabular}             & \begin{tabular}[c]{@{}c@{}}정부 (86)\\Government\\(jeongbu)\end{tabular}                                       & \begin{tabular}[c]{@{}c@{}}우크라이나 (17)\\Ukraine\\(ukeuraina)\end{tabular}                                     \\ 
\hline
17 & \begin{tabular}[c]{@{}c@{}}안 (37)\\Last name of some\\politicians or Not\\(an)\end{tabular}                     & \begin{tabular}[c]{@{}c@{}}한다. (66)\\Do\\(handa)\end{tabular}                                                    & \begin{tabular}[c]{@{}c@{}}대통령 (74)\\President\\(daetongryeong)\end{tabular}                                & \begin{tabular}[c]{@{}c@{}}이재명 (85)\\Name of a\\politician\\(ijaemyeong)\end{tabular}                        & \begin{tabular}[c]{@{}c@{}}의원은 (17)\\Member of a legislative assembly is\\(uiwoneun)\end{tabular}            \\ 
\hline
18 & \begin{tabular}[c]{@{}c@{}}대통령의 (36)\\Presidential\\(daetongryeongui)\end{tabular}                              & \begin{tabular}[c]{@{}c@{}}안 (65)\\Last name of some\\politicians or Not\\(an)\end{tabular}                      & \begin{tabular}[c]{@{}c@{}}일본 (70)\\Japan\\(ilbon)\end{tabular}                                             & \begin{tabular}[c]{@{}c@{}}밝혔다. (84)\\Revealed\\(balkhyeossda)\end{tabular}                                  & \begin{tabular}[c]{@{}c@{}}중국 (17)\\China\\(jungguk)\end{tabular}                                            \\ 
\hline
19 & \begin{tabular}[c]{@{}c@{}}지적했다. (33)\\Pointed out\\(jijeokhaessda)\end{tabular}                                & \begin{tabular}[c]{@{}c@{}}대통령의 (64)\\Presidential\\(daetongryeongui)\end{tabular}                               & \begin{tabular}[c]{@{}c@{}}국민의힘 (69)\\The full name of Korea conservative party\\(gukminuihim)\end{tabular} & \begin{tabular}[c]{@{}c@{}}대표가 (83)\\Representative is \\(daepyoga)\end{tabular}                             & \begin{tabular}[c]{@{}c@{}}서울 (16)\\Seoul\\(seoul)\end{tabular}                                              \\ 
\hline
20 & \begin{tabular}[c]{@{}c@{}}더불어민주당 (33)\\The full name of Korea liberal party \\(deobureominjudang)\end{tabular} & \begin{tabular}[c]{@{}c@{}}당 (61)\\Party\\(dang)\end{tabular}                                                    & \begin{tabular}[c]{@{}c@{}}국회 (68)\\National assembly\\(gukhoe)\end{tabular}                                & \begin{tabular}[c]{@{}c@{}}국회 (82)\\National assembly\\(gukhoe)\end{tabular}                                 & \begin{tabular}[c]{@{}c@{}}민주당은 (16)\\Korea liberal party is\\(minjudang)\end{tabular}                       \\ 
\hline
\end{tabular}
\end{adjustbox}
\caption{Top20 of word frequency about political orientation (Task1). List of most frequent words for each class: We show Korean words(count) and translation in English(Romanizing Korean pronunciation)}
\label{word_frequency_table}
\end{table}
\vspace{30pt}

We calculate word frequency by breaking down the article into individual sentences. We exclude subjects with unclear targets like "He", prepositions like "About" and "For", and conjunctions like "And". We extract word frequencies by utilizing the algorithm.

\begin{table}[h]
\centering
 % Adjusting the row spacing
\begin{adjustbox}{width=\textwidth}
\begin{tabular}{|c|c|c|c|c|c|c|} 
\hline
   & \multicolumn{6}{c|}{The level of Pro-Government}                                                                                                                                    \\ 
\cline{2-7}

 Rank   & class 0                                                                                                          & class 1                                                                                                         & class 2                                                                                                         & class 3                                                                                           & class 4                                                                                                     & class 5                                                                                          \\ 
\hline
1  & \begin{tabular}[c]{@{}c@{}}전 (445)\\Ex \\(jeon)\end{tabular}                                                     & \begin{tabular}[c]{@{}c@{}}이 (204)\\Last name of some\\politicians or This\\(Yi)\end{tabular}                   & \begin{tabular}[c]{@{}c@{}}전 (115)\\Ex \\(jeon)\end{tabular}                                                    & \begin{tabular}[c]{@{}c@{}}전 (106)\\Ex \\(jeon)\end{tabular}                                      & \begin{tabular}[c]{@{}c@{}}윤 (161)\\Last name of some\\politicians \\(yun)\end{tabular}                     & \begin{tabular}[c]{@{}c@{}}윤 (153)\\Last name of some\\politicians \\(yun)\end{tabular}          \\ 
\hline
2  & \begin{tabular}[c]{@{}c@{}}이 (414)\\Last name of some\\politicians or This\\(Yi)\end{tabular}                    & \begin{tabular}[c]{@{}c@{}}있다. (178)\\be \\(issda)\end{tabular}                                                 & \begin{tabular}[c]{@{}c@{}}있다. (97)\\be \\(issda)\end{tabular}                                                  & \begin{tabular}[c]{@{}c@{}}있다. (106)\\be \\(issda)\end{tabular}                                   & \begin{tabular}[c]{@{}c@{}}했다. (157)\\did \\(haessda)\end{tabular}                                          & \begin{tabular}[c]{@{}c@{}}대통령은 (149)\\President is \\(daetongryeongeun)\end{tabular}            \\ 
\hline
3  & \begin{tabular}[c]{@{}c@{}}했다. (302)\\did \\(haessda)\end{tabular}                                               & \begin{tabular}[c]{@{}c@{}}윤 (172)\\Last name of some\\politicians \\(yun)\end{tabular}                         & \begin{tabular}[c]{@{}c@{}}했다. (90)\\did \\(haessda)\end{tabular}                                               & \begin{tabular}[c]{@{}c@{}}했다. (94)\\did \\(haessda)\end{tabular}                                 & \begin{tabular}[c]{@{}c@{}}말했다. (103)\\Said \\(malhaessda)\end{tabular}                                     & \begin{tabular}[c]{@{}c@{}}했다. (111)\\did \\(haessda)\end{tabular}                               \\ 
\hline
4  & \begin{tabular}[c]{@{}c@{}}있다. (286)\\be \\(issda)\end{tabular}                                                  & \begin{tabular}[c]{@{}c@{}}윤석열 (163)\\Name of Korea\\president\\(yunseogyeol)\end{tabular}                      & \begin{tabular}[c]{@{}c@{}}이 (83)\\Last name of some\\politicians or This\\(Yi)\end{tabular}                    & \begin{tabular}[c]{@{}c@{}}윤 (91)\\Last name of some\\politicians \\(yun)\end{tabular}            & \begin{tabular}[c]{@{}c@{}}대통령은 (102)\\President is \\(daetongryeongeun)\end{tabular}                       & \begin{tabular}[c]{@{}c@{}}윤석열 (49)\\Name of Korea\\president\\(yunseogyeol)\end{tabular}        \\ 
\hline
5  & \begin{tabular}[c]{@{}c@{}}대표는 (208) \\Representative is \\(daepyoneun)\end{tabular}                             & \begin{tabular}[c]{@{}c@{}}전 (162)\\Ex \\(jeon)\end{tabular}                                                    & \begin{tabular}[c]{@{}c@{}}오염수 (65)\\Contaminated water (oyeomsu)\end{tabular}                                  & \begin{tabular}[c]{@{}c@{}}윤석열 (80)\\Name of Korea\\president\\(yunseogyeol)\end{tabular}         & \begin{tabular}[c]{@{}c@{}}있다. (99)\\be \\(issda)\end{tabular}                                              & \begin{tabular}[c]{@{}c@{}}대통령이 (40)\\President is (daetongryeongi)\end{tabular}                 \\ 
\hline
6  & \begin{tabular}[c]{@{}c@{}}의원은 (195)\\Member of a legislative assembly is\\(uiwoneun)\end{tabular}               & \begin{tabular}[c]{@{}c@{}}했다. (161)\\did \\(haessda)\end{tabular}                                              & \begin{tabular}[c]{@{}c@{}}홍 (53)\\Last name of some\\politicians \\(hong)\end{tabular}                         & \begin{tabular}[c]{@{}c@{}}대통령은 (69)\\President is \\(daetongryeongeun)\end{tabular}              & \begin{tabular}[c]{@{}c@{}}전 (91)\\Ex \\(jeon)\end{tabular}                                                 & \begin{tabular}[c]{@{}c@{}}말했다. (31)\\Said \\(malhaessda)\end{tabular}                           \\ 
\hline
7  & \begin{tabular}[c]{@{}c@{}}김 (179)\\Last name of some\\politicians\\(kim)\end{tabular}                           & \begin{tabular}[c]{@{}c@{}}대통령이 (124)\\President is (daetongryeongi)\end{tabular}                               & \begin{tabular}[c]{@{}c@{}}말했다. (46)\\Said \\(malhaessda)\end{tabular}                                          & \begin{tabular}[c]{@{}c@{}}대통령이 (61)\\President is (daetongryeongi)\end{tabular}                  & \begin{tabular}[c]{@{}c@{}}이 (87)\\Last name of some\\politicians or This\\(Yi)\end{tabular}                & \begin{tabular}[c]{@{}c@{}}대통령실 (30)\\Office of the president\\(daetongryeongsil )\end{tabular}  \\ 
\hline
8  & \begin{tabular}[c]{@{}c@{}}민주당 (178)\\The name of Korea liberal party \\(minjudang)\end{tabular}                 & \begin{tabular}[c]{@{}c@{}}대통령의 (109)\\Presidential\\(daetongryeongui)\end{tabular}                             & \begin{tabular}[c]{@{}c@{}}일본 (45)\\Japan\\(ilbon)\end{tabular}                                                 & \begin{tabular}[c]{@{}c@{}}말했다. (52)\\Said \\(malhaessda)\end{tabular}                            & \begin{tabular}[c]{@{}c@{}}윤석열 (71)\\Name of Korea\\president\\(yunseogyeol)\end{tabular}                   & \begin{tabular}[c]{@{}c@{}}우크라이나 (30)\\Ukraine\\(ukeuraina)\end{tabular}                         \\ 
\hline
9  & \begin{tabular}[c]{@{}c@{}}대표가 (156)\\Representative is \\(daepyoga)\end{tabular}                                & \begin{tabular}[c]{@{}c@{}}김 (100)\\Last name of some\\politicians\\(kim)\end{tabular}                          & \begin{tabular}[c]{@{}c@{}}국민의힘 (39)\\The full name of Korea conservative party\\(gukminuihim)\end{tabular}     & \begin{tabular}[c]{@{}c@{}}열린 (51)\\Open\\(yeollin)\end{tabular}                                  & \begin{tabular}[c]{@{}c@{}}김 (66)\\Last name of some\\politicians\\(kim)\end{tabular}                       & \begin{tabular}[c]{@{}c@{}}대통령 (28)\\President\\(daetongryeong)\end{tabular}                     \\ 
\hline
10 & \begin{tabular}[c]{@{}c@{}}국민의힘 (154)\\The full name of Korea conservative party\\(gukminuihim)\end{tabular}     & \begin{tabular}[c]{@{}c@{}}말했다. (96)\\Said \\(malhaessda)\end{tabular}                                          & \begin{tabular}[c]{@{}c@{}}한국 (38)\\Korea\\(hanguk)\end{tabular}                                                & \begin{tabular}[c]{@{}c@{}}의원은 (49)\\Member of a legislative assembly is\\(uiwoneun)\end{tabular} & \begin{tabular}[c]{@{}c@{}}밝혔다. (55)\\Revealed\\(balkhyeossda)\end{tabular}                                 & \begin{tabular}[c]{@{}c@{}}있다. (26)\\be \\(issda)\end{tabular}                                   \\ 
\hline
11 & \begin{tabular}[c]{@{}c@{}}말했다. (151)\\Said \\(malhaessda)\end{tabular}                                          & \begin{tabular}[c]{@{}c@{}}대통령은 (84)\\President is \\(daetongryeongeun)\end{tabular}                            & \begin{tabular}[c]{@{}c@{}}의원은 (36)\\Member of a legislative assembly is\\(uiwoneun)\end{tabular}               & \begin{tabular}[c]{@{}c@{}}이 (44)\\Last name of some\\politicians or This\\(Yi)\end{tabular}      & \begin{tabular}[c]{@{}c@{}}대통령이 (53)\\President is \\(daetongryeongi)\end{tabular}                          & \begin{tabular}[c]{@{}c@{}}정부 (25)\\Government\\(jeongbu)\end{tabular}                           \\ 
\hline
12 & \begin{tabular}[c]{@{}c@{}}이재명 (148)\\Name of a\\politician\\(ijaemyeong)\end{tabular}                           & \begin{tabular}[c]{@{}c@{}}대표는 (83)\\Representative is \\(daepyoneun)\end{tabular}                              & \begin{tabular}[c]{@{}c@{}}김 (34)\\Last name of some\\politicians\\(kim)\end{tabular}                           & \begin{tabular}[c]{@{}c@{}}대통령 (41)\\President\\(daetongryeong)\end{tabular}                      & \begin{tabular}[c]{@{}c@{}}장관은 (51)\\Minister is\\(janggwaneun)\end{tabular}                                & \begin{tabular}[c]{@{}c@{}}싱 (24)\\Last name of the Chinese ambassador\\(xing)\end{tabular}      \\ 
\hline
13 & \begin{tabular}[c]{@{}c@{}}국회 (144)\\National assembly\\(gukhoe)\end{tabular}                                    & \begin{tabular}[c]{@{}c@{}}의원은 (77)\\Member of a legislative assembly is\\(uiwoneun)\end{tabular}               & \begin{tabular}[c]{@{}c@{}}민주당 (34)\\The name of Korea liberal party \\(minjudang)\end{tabular}                 & \begin{tabular}[c]{@{}c@{}}북한 (40)\\North Korea\\(bukhan)\end{tabular}                            & \begin{tabular}[c]{@{}c@{}}국민의힘 (50)\\The full name of Korea conservative party\\(gukminuihim)\end{tabular} & \begin{tabular}[c]{@{}c@{}}이 (20)\\Last name of some\\politicians or This\\(Yi)\end{tabular}     \\ 
\hline
14 & \begin{tabular}[c]{@{}c@{}}당 (135)\\Party\\(dang)\end{tabular}                                                   & \begin{tabular}[c]{@{}c@{}}대통령 (74)\\President\\(daetongryeong)\end{tabular}                                    & \begin{tabular}[c]{@{}c@{}}윤 (33)\\Last name of some\\politicians \\(yun)\end{tabular}                          & \begin{tabular}[c]{@{}c@{}}김 (40)\\Last name of some\\politicians\\(kim)\end{tabular}             & \begin{tabular}[c]{@{}c@{}}오염수 (48)\\Contaminated water\\(oyeomsu)\end{tabular}                             & \begin{tabular}[c]{@{}c@{}}지원 (19)\\Support\\(jiwon)\end{tabular}                                \\ 
\hline
15 & \begin{tabular}[c]{@{}c@{}}더불어민주당 (127)\\The full name of Korea liberal party \\(deobureominjudang)\end{tabular} & \begin{tabular}[c]{@{}c@{}}비판했다. (71)\\Criticized \\(bipanhaessda)\end{tabular}                                 & \begin{tabular}[c]{@{}c@{}}윤석열 (32)\\Name of Korea\\president\\(yunseogyeol)\end{tabular}                       & \begin{tabular}[c]{@{}c@{}}오염수 (39)\\Contaminated water\\(oyeomsu)\end{tabular}                   & \begin{tabular}[c]{@{}c@{}}정부 (47)\\Government\\(jeongbu)\end{tabular}                                      & \begin{tabular}[c]{@{}c@{}}열린 (18)\\Open\\(yeollin)\end{tabular}                                 \\ 
\hline
16 & \begin{tabular}[c]{@{}c@{}}의원 (101)\\Member of a legislative assembly\\(uiwon)\end{tabular}                      & \begin{tabular}[c]{@{}c@{}}안 (68)\\Last name of some\\politicians or Not\\(an)\end{tabular}                     & \begin{tabular}[c]{@{}c@{}}시장은 (31)\\Mayor\\(sijangeun)\end{tabular}                                            & \begin{tabular}[c]{@{}c@{}}일본 (38)\\Japan\\(ilbon)\end{tabular}                                   & \begin{tabular}[c]{@{}c@{}}후쿠시마 (44)\\Fukushima City\\(hukusima)\end{tabular}                               & \begin{tabular}[c]{@{}c@{}}김 (18)\\Last name of some\\politicians\\(kim)\end{tabular}            \\ 
\hline
17 & \begin{tabular}[c]{@{}c@{}}열린 (95)\\Open\\(yeollin)\end{tabular}                                                 & \begin{tabular}[c]{@{}c@{}}민주당 (67)\\The name of Korea liberal party \\(minjudang)\end{tabular}                 & \begin{tabular}[c]{@{}c@{}}안 (28)\\Last name of some\\politicians or Not\\(an)\end{tabular}                     & \begin{tabular}[c]{@{}c@{}}부산 (37)\\Busan city\\(busan)\end{tabular}                              & \begin{tabular}[c]{@{}c@{}}함께 (43)\\Together\\(hamkke)\end{tabular}                                         & \begin{tabular}[c]{@{}c@{}}전 (17)\\Ex \\(jeon)\end{tabular}                                      \\ 
\hline
18 & \begin{tabular}[c]{@{}c@{}}밝혔다. (92)\\Revealed\\(balkhyeossda)\end{tabular}                                      & \begin{tabular}[c]{@{}c@{}}밝혔다. (65)\\Revealed\\(balkhyeossda)\end{tabular}                                     & \begin{tabular}[c]{@{}c@{}}정부 (27)\\Government\\(jeongbu)\end{tabular}                                          & \begin{tabular}[c]{@{}c@{}}27일 (35)\\27th-date\\(isipchiril)\end{tabular}                         & \begin{tabular}[c]{@{}c@{}}일본 (41)\\Japan\\(ilbon)\end{tabular}                                             & \begin{tabular}[c]{@{}c@{}}중국 (17)\\China\\(jungguk)\end{tabular}                                \\ 
\hline
19 & \begin{tabular}[c]{@{}c@{}}대표 (86)\\Representative\\(daepyo)\end{tabular}                                        & \begin{tabular}[c]{@{}c@{}}정부의 (63)\\Of government\\(jeongbuui)\end{tabular}                                    & \begin{tabular}[c]{@{}c@{}}정부가 (25)\\Government is\\(jeongbuga)\end{tabular}                                    & \begin{tabular}[c]{@{}c@{}}유엔군 (33)\\The UN forces\\(yuengun)\end{tabular}                        & \begin{tabular}[c]{@{}c@{}}관계자는 (40)\\An official is\\(gwangyejaneun)\end{tabular}                          & \begin{tabular}[c]{@{}c@{}}한다"고 (17)\\To do\\(handago)\end{tabular}                              \\ 
\hline
20 & \begin{tabular}[c]{@{}c@{}}서울 (86)\\Seoul\\(seoul)\end{tabular}                                                  & \begin{tabular}[c]{@{}c@{}}더불어민주당 (61)\\The full name of Korea liberal party \\(deobureominjudang)\end{tabular} & \begin{tabular}[c]{@{}c@{}}감사원 (25)\\The Board of Audit and Inspection\\(gamsawon)\end{tabular}                 & \begin{tabular}[c]{@{}c@{}}기자 (32)\\Journalist\\(gija)\end{tabular}                               & \begin{tabular}[c]{@{}c@{}}국회 (39)\\National assembly\\(gukhoe)\end{tabular}                                & \begin{tabular}[c]{@{}c@{}}보조금 (17)\\Subsidy\\(bojogeum)\end{tabular}                            \\ 
\hline
\end{tabular}
\end{adjustbox}
\caption{Top20 of word frequency about the level of pro-government (Task2). List of most frequent words for each class: We show Korean words(count) and translation in English(Romanizing Korean pronunciation)}
\label{word_frequency_table}
\end{table}

In the Korean language, one can often observe the frequent use of particles, demonstrative pronouns, and surnames. Particularly, verbs used for quotations such as "said" and "is" were commonly found across all labels. Nonetheless, there were notable similarities among the high-frequency vocabulary for each label. For labels leaning towards the progressive side, surnames or names of progressive figures were more common, while on the conservative side, names or surnames of conservative figures were more prevalent. Additionally, for the progressive-leaning labels, words with aggressive tones such as "criticism" or "pointing out" were more frequent, whereas for the conservative-leaning labels, criticisms of the previous administration and vocabulary supporting the current government were ranked higher.

\clearpage
\section{Total Results When Tested Non-uniformly}

\begin{table}[!htb]
    \centering
    \begin{adjustbox}{width=\textwidth}
     % Adjusting the row spacing
    \begin{tabular}{c|c|c|c|c|c|c|c|c}
        \hline
        \multicolumn{2}{c|}{\textbf{Model}} & \textbf{Top-2 Accuracy} & \textbf{Accuracy} & \textbf{F1-macro} & \textbf{F1-micro} & \textbf{F1-weighted} & \textbf{MAE} & \textbf{Hamming Loss}\\
        \hline
        \multirow{2}{*}{KoPolitic} & Task1 & 0.8147 & 0.6355 & 0.5530 & 0.6355 & 0.6313 & 0.4880 & 0.3645 \\
        \cline{2-9}
        & Task2 & 0.8367 & 0.6295 & 0.5406 & 0.6295 & 0.6241 & 0.7410 & 0.3705 \\
        \hline
    \end{tabular}
    \end{adjustbox}
    \caption{Performance metrics for KoPolitic tasks evaluated on a test dataset aligned with real-world data distribution. Metrics include Top-2 accuracy, accuracy, F1-score macro, F1-micro, F1-weighted, MAE, and Hamming Loss.}
    \label{ununiformed_results}
\end{table}

\begin{figure}[!htb]
    \includegraphics[width=\textwidth]{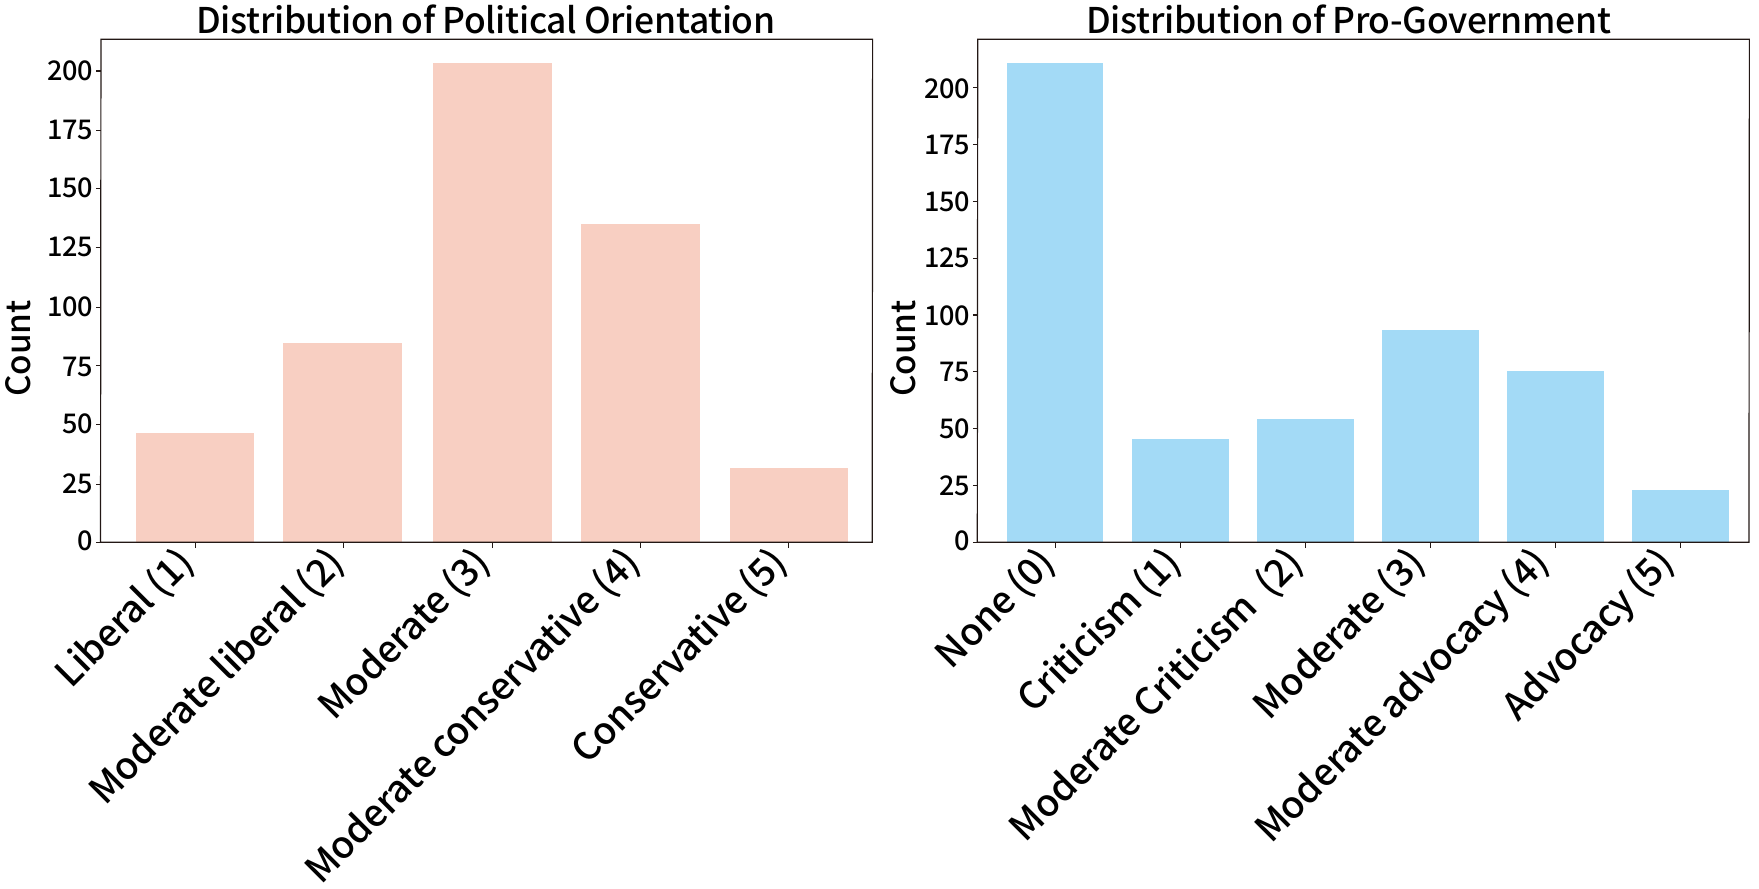}
    \caption{Test Dataset Distribution Aligned with Real-World Data Distribution}
    \label{fig:model_configuration}
\end{figure}

\begin{figure}[!htb]
    \includegraphics[width=\textwidth]{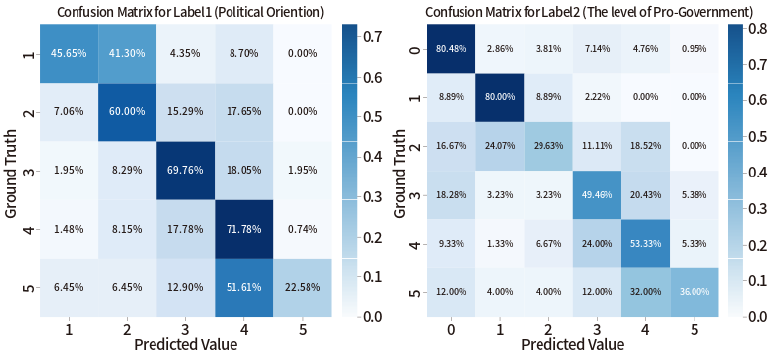}
    \caption{Confusion Matrix from Evaluating a Non-Uniformly Distributed Test Dataset}
    \label{fig:model_configuration}
\end{figure}

When evaluated with non-uniform test data, Top-2 accuracy, accuracy, and F1-score (macro, micro, weighted) all increased, while MAE and Hamming Loss both decreased.

\clearpage
\section{Original Articles from the Model Illustration}
\begin{figure}[!htb]
    \includegraphics[width=\textwidth]{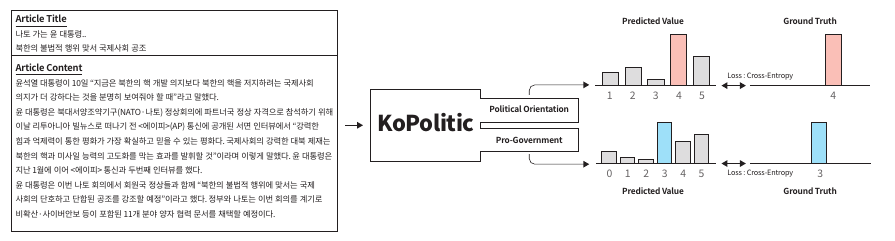}
    \caption{The conceptual illustration of our proposed model with the original data input and output examples. We note that our proposed architecture simultaneously predicts two types of outputs, (1) political orientation and (2) the level of attitude towards government utilizing multi-task learning loss.}
    \label{fig:model_image_korean}
\end{figure}

\section{Data Collection Source}
\begin{table}[h]
\centering
\begin{tabular}{|c|c|c|}
\hline
\multicolumn{1}{|c|}{\textbf{Political Orientation}} & \textbf{Newspaper} & \textbf{Link} \\
\hline
\multirow{2}{*}{Conservative leaning} & 조선일보 (Chosunilbo) & www.chosun.com \\
& 중앙일보 (Joongangilbo) & www.joongang.co.kr \\
\hline
\multirow{2}{*}{Neutral leaning} & 연합뉴스 (Yonhapnews) & www.yna.co.kr \\
& 뉴스1 (News 1) & www.news1.kr \\
\hline
\multirow{2}{*}{Liberal leaning} & 한겨레 (Hanyoreh) & www.hani.co.kr \\
& 프레시안 (Pressian)  & www.pressian.com \\
\hline
\end{tabular}
\caption{Data Collection Source. We have collected a total of 12,000 political articles from two conservative-leaning newspapers, two neutral-leaning newspapers, and two liberal-leaning newspapers, representing prominent media outlets in South Korea.}
\label{data_sources}
\end{table}

%%% Local Variables:
%%% mode: latex
%%% TeX-master: t
%%% End:
